# Supplementary material for: Nanocavity-mediated Purcell enhancement of Er in TiO$_2$ thin films grown via atomic layer deposition
Source: arXiv:2309.13490 ancillary file (2023-09-23)
Supplement: Supplementary file 1 [file SI_Nanocavity-mediated_Purcell_enhancement_of_Er_in_TiO_2_thin_films_grown_via_atomic_layer_deposition.pdf]

Supporting Information for

**Nanocavity-mediated Purcell enhancement of Er in TiO<sub>2</sub> thin  
films grown via atomic layer deposition**

Cheng Ji,<sup>†,‡</sup> Michael T. Solomon,<sup>†,‡,¶</sup> Gregory D. Grant,<sup>†,‡</sup> Koichi Tanaka,<sup>†</sup> Muchuan Hua,<sup>§</sup>  
Jianguo Wen,<sup>§</sup> Sagar K. Seth,<sup>†,‡</sup> Connor P. Horn,<sup>†,‡</sup> Ignas Masiulionis,<sup>†,‡</sup> Manish K.  
Singh,<sup>†,⊥</sup> Sean E. Sullivan,<sup>‡,¶,⊥</sup> F. Joseph Heremans,<sup>‡,¶,†</sup> David D. Awschalom,<sup>†,‡,¶,||</sup>  
Supratik Guha,<sup>\*,†,‡,¶</sup> and Alan M. Dibos<sup>\*,§,¶</sup>

<sup>†</sup>*Pritzker School of Molecular Engineering, University of Chicago, Chicago, IL 60637*

<sup>‡</sup>*Materials Science Division, Argonne National Laboratory, Lemont, IL 60439*

<sup>¶</sup>*Center for Molecular Engineering, Argonne National Laboratory, Lemont, IL 60439*

<sup>§</sup>*Nanoscience and Technology Division, Argonne National Laboratory, Lemont, IL 60439*

<sup>||</sup>*Department of Physics, University of Chicago, Chicago, IL 60637*

<sup>⊥</sup>*Current address: memQ Inc., Chicago, IL 60615*

E-mail: sguha@anl.gov; adibos@anl.gov

# 1 Surface morphology from higher substrate temperature ALD $\text{TiO}_2$ growth

In contrast to the low growth temperature and annealed  $\text{Er}:\text{TiO}_2$  samples primarily explored in this work, we have performed AFM height maps on a  $2\text{ }\mu\text{m} \times 2\text{ }\mu\text{m}$  area for an undoped, unannealed  $\text{TiO}_2$  film grown with a Si substrate temperature of  $300\text{ }^\circ\text{C}$  (Fig. S1). The total thickness of the film is approximately 20 nm and the growth rate is similar to that of the thin films shown in Figure 1c-d in the main text. The resultant roughness (3-4 nm) suggests that  $\text{TiO}_2$  ALD growth in a higher substrate temperature regime (amenable to direct crystal formation) yields much rougher films than those that are amorphous after growth at  $120\text{ }^\circ\text{C}$  and ex-situ annealed at  $400\text{ }^\circ\text{C}$ .

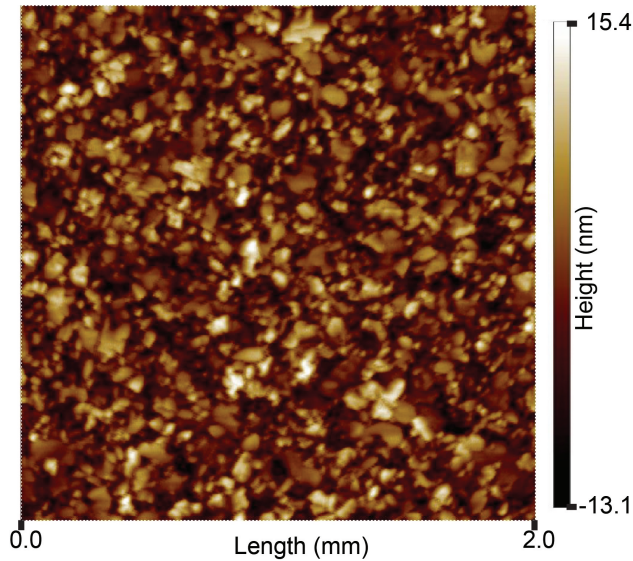

**Figure S1: AFM scan of high deposition temperature.** AFM scan of an undoped and unannealed  $\text{TiO}_2$  film grown with a substrate temperature of  $300\text{ }^\circ\text{C}$ . The  $R_a$  and  $R_q$  values are 4.43 nm and 3.62 nm, respectively.

## 2 TEM elemental mapping

In order to corroborate our HAADF-STEM results showing increased brightness in the nominally Er-doped region within the ‘20/50/20’ heterostructure (Fig. 2 of the main text), we also performed TEM energy dispersive x-ray spectroscopy (EDS). Figure S2 shows an overlay of the Si, Ti, and Er elemental distributions within the heterostructure. The band of

bright green (corresponding to the Er-rich area) within the ‘20/50/20’ sandwich atop the Si substrate is clearly shown.

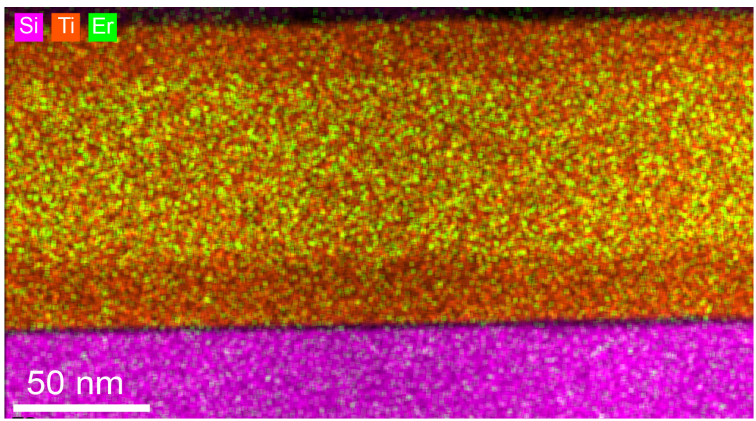

**Figure S2: Energy-dispersive X-ray spectroscopy (EDS) elemental map.** An overlay of the elemental distribution of Si, Ti, and Er (shown in purple, orange, and green, respectively).

### 3 HAADF-STEM of as-grown vs annealed samples

We also performed HAADF-STEM imaging of as-grown versus 400 °C annealed samples (Fig. S3). These cross-sections are prepared from the same growth film (Er doping level of 39200 ppm) and both images are near the undoped-doped interface closer to the substrate. The as-grown film is completely amorphous without regularity in the single atom spacing (Fig. S3a). In contrast, the 400 °C annealed thin film clearly shows the regular lattice spacing for a single crystal anatase domain that dominates the entire field of view (Fig. S3b).

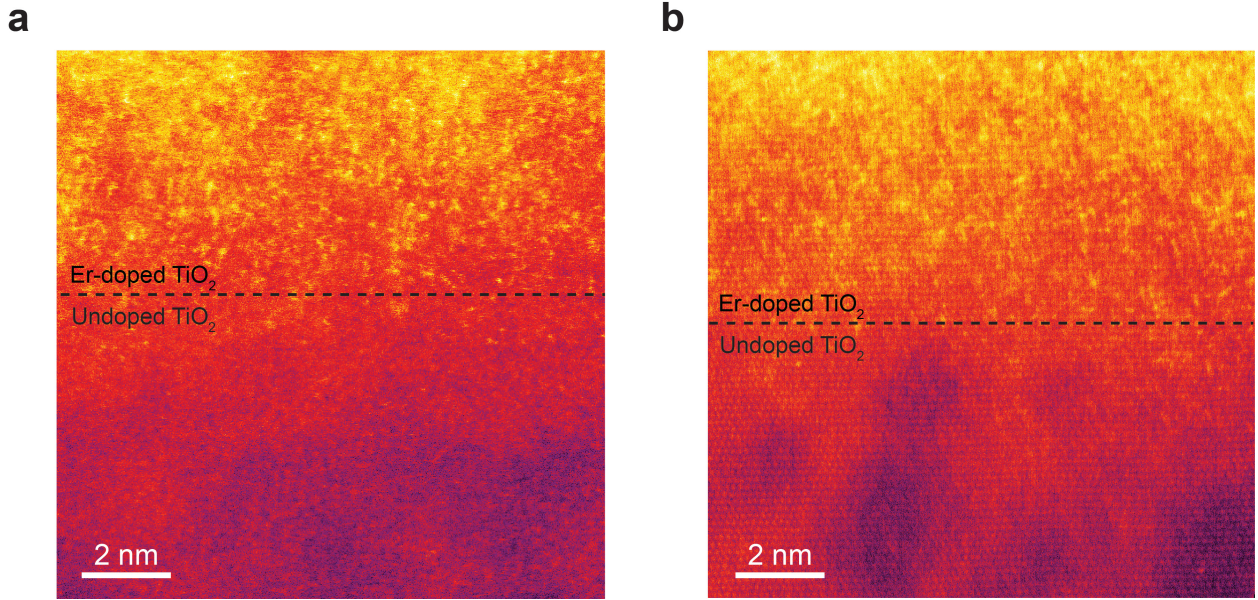

**Figure S3: High-angle annular dark-field (HAADF) STEM images before and after annealing.** (a) HAADF-STEM images of a cross section of an as-grown ‘20/50/20’ sample. (b) A different piece from the same growth sample as in (a) after oxygen annealing. The doping level of the growth sample is 39200 ppm.

## 4 Additional EBSD mapping on thinner heterostructures

We wanted to investigate if there are differences in the overall grain structure for the thinner ‘10/10/10’ heterostructures used for thin film and device optical measurements versus the thicker ‘20/50/20’ films shown in Figure 2d of the main text. In Figure S4, we show additional EBSD phase maps for the ‘10/10/10’ thin film with 2950 ppm Er doping after oxygen annealing. While they are similar in nature, we can see that the phase map at 10 kV (Fig. S4a) for the ‘10/10/10’ heterostructure has higher anatase grain coverage than the 10 kV map for the ‘20/50/20’ sample shown in Figure 2d of the main text. We do not know the exact effective sampling depth at this voltage for our polycrystalline samples; however, we speculate that the higher percentage of anatase grains detected may be because the overall thinner  $\text{TiO}_2$  film can lead to increased anatase grain coarsening rather than vertical stacking of grains. If we also use a higher accelerating voltage of 20 kV on the ‘10/10/10’ heterostructure (for a nearby but distinct scan area from Fig. S4a because of electron beam damage), we see a dramatic reduction in the anatase grains detected (Fig. S4). This is

primarily because EBSD lateral resolution of grains and overall penetration depth are highly dependent on accelerating voltage, with higher voltage probing deeper into the sample.<sup>1</sup> At 20 kV we see electron diffraction patterns from the underlying Si substrate as well as the anatase  $\text{TiO}_2$  leading to the predominant black color in the resultant grain map (Fig. S4b). However, the results on the 30 nm thick film still demonstrate that the anatase grains can extend for hundreds of nanometers laterally and it is possible that these grains span the entire thickness of the  $\text{TiO}_2$  layer.

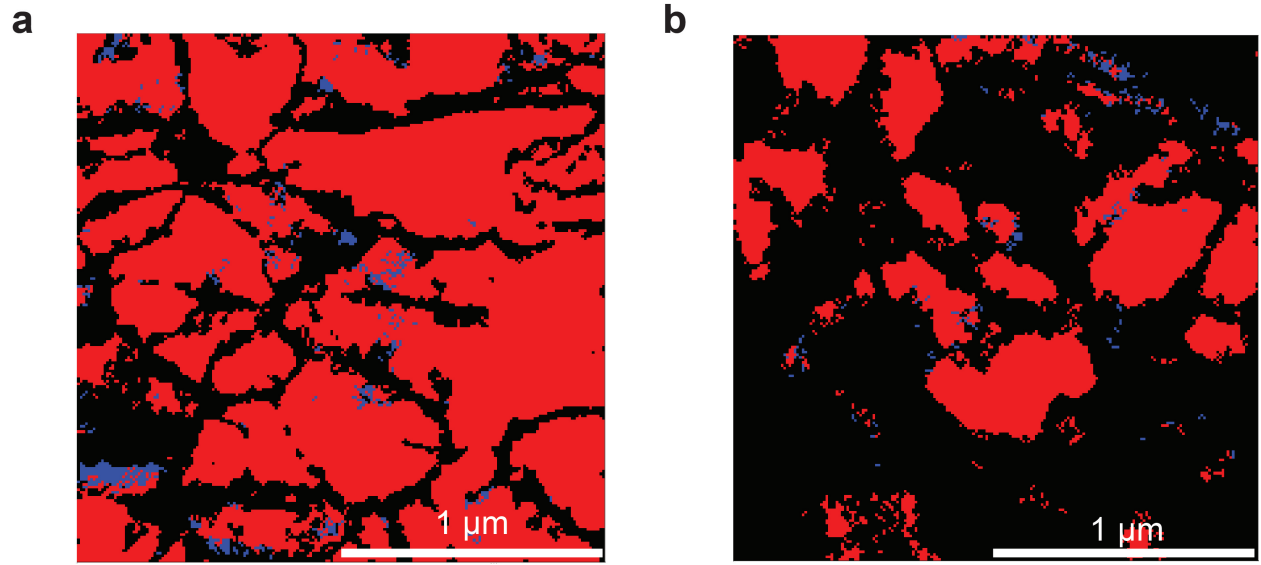

**Figure S4: Electron backscatter diffraction (EBSD) phase map of individual grains for ‘10/10/10’ thin film samples.** (a) EBSD phase map with operation voltage at 10 kV, showing 66.7% anatase grains and 1.9% rutile grains. (b) EBSD results with operation voltage at 20 kV, showing 23.9% anatase grains and 0.8% rutile grains.

## 5 Optical measurement configurations

In this work, we employ two separate optical measurement configurations to characterize the ALD  $\text{Er}:\text{TiO}_2$  properties. The first optical setup is a cryogenic confocal microscope designed and optimized for thin film PLE measurements<sup>2</sup> (Figure S4a), and the second one is designed for lensed optical fiber end-fire coupling to fabricated nanophotonic devices,<sup>3</sup> (Figure S5b). The hardware details of each configuration are delineated in the *Methods* section of the main text.

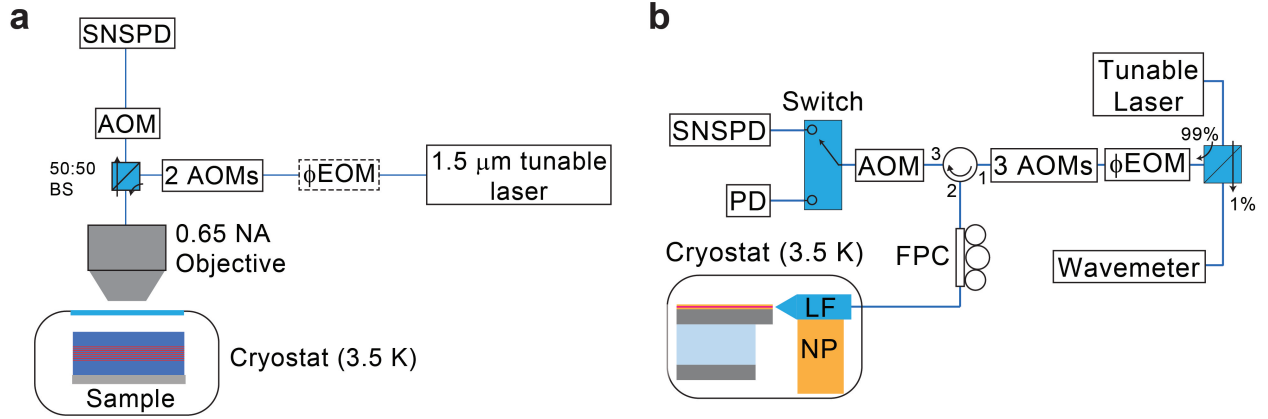

**Figure S5: The optical setup.** (a) the optical measurement setup for the thin films. (b) the optical measurement setup for the fabricated nanophotonic devices. AOM: acousto-optic modulator, FPC: fiber polarization controller,  $\phi\text{EOM}$ : electro-optic phase modulator, PD: amplified photodiode, SNSPD: superconducting nanowire single-photon detector.

## 6 PLE on an as-grown versus unannealed sample

In order to compare the as-grown and annealed thin film optical emission, we also measured the PLE spectrum for the as-grown  $\text{Er}:\text{TiO}_2$  thin film with a doping level of 39200 ppm. The as-grown PLE (dashed line) is shown in Figure S6 as compared with the solid red line (reproduced from Figure 3 of the main text). The as-grown PLE spectrum did not show any emission peaks and the brightness of the emission was close to the background level. This measurement confirms that the oxygen annealing process is essential to not only form crystalline grains within the sample but also to optically "activate" the embedded Er ions.

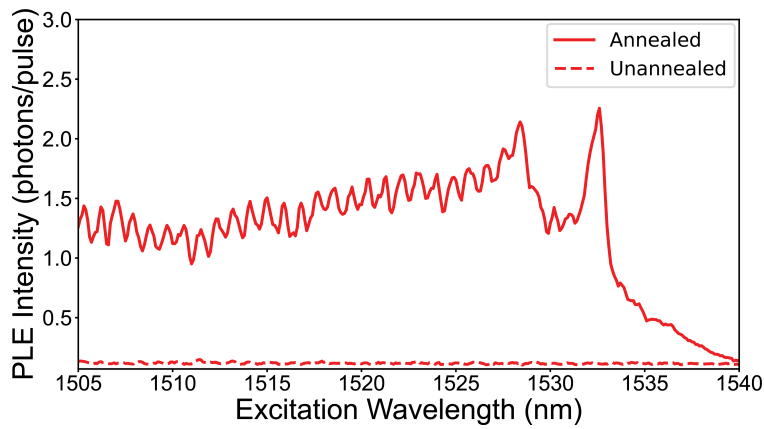

**Figure S6: PLE spectra of annealed versus as-grown 10/10/10  $\text{Er}:\text{TiO}_2$  thin film.** The Er doping concentration of the film is 39200 ppm, corresponding to the condition No.1 in Table 1 of the main text. The annealed sample PLE spectrum is shown in solid red lines while the unannealed sample from the same growth wafer is shown in red dashed line.

## 7 PLE scan on 1.7 ppm waveguide-based device

As mentioned in the main text, thin film confocal PLE measurements on the 1.7 ppm Er-doped sample are challenging due to low signal. We are forced to pump at high laser intensity, and as a result, the peaks shown in Figure 3c (inset) are power-broadened. Therefore, we have also performed a PLE scan using a waveguide device with a non-resonant cavity. In particular, this device is selected because its as-fabricated cavity resonance is detuned to 1522 nm, such that the cavity acts as a mirror for photons emitted by the embedded Er ions along the waveguide for improved collection efficiency. Because of the improved coupling efficiency and increased optical depth of the waveguide devices, our signal-to-noise ratio is better and a two-order of magnitude lower laser pump power can be used. The resultant PLE scan at 3.1 K is shown in Figure S7, which gives a Lorentzian fit of  $44.0 \pm 0.7$  GHz for the peak at 1532.6 nm. This suggests the inhomogeneous linewidth for this sample is closer to this range instead of the 102.2 GHz shown in Figure 3c of the main text.

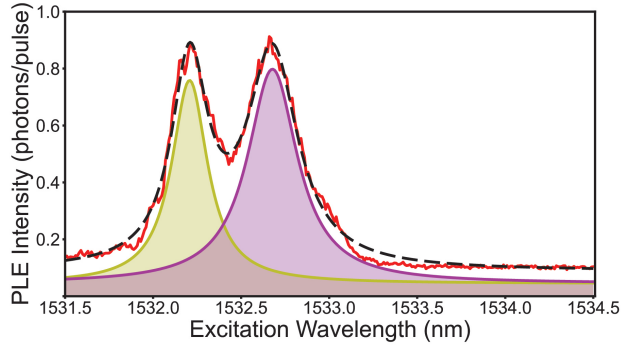

**Figure S7: PLE scan of an annealed 10/10/10 Er:TiO<sub>2</sub> thin film with 1.7 ppm doping via a waveguide device.** The PLE scan shows two peaks near 1532.2 and 1532.6 nm. The peak at 1532.6 nm gives an inhomogeneous linewidth of the emission peak of  $44.0 \pm 0.7$  GHz via Lorentzian fits.

## References

- (1) Wisniewski, W.; Saager, S.; Böbenroth, A.; Rüssel, C. Experimental evidence concerning the significant information depth of electron backscatter diffraction (EBSD). *Ultramicroscopy* **2017**, *173*, 1–9.
- (2) Ji, C.; Grant, G. D.; Singh, M. K.; Seth, S.; Tanaka, K.; Dibos, A. M.; Guha, S. Optical properties of Er ion doped TiO<sub>2</sub> with atomic layer deposition. Quantum Information Science, Sensing, and Computation XV. 2023; p 1251702.
- (3) Dibos, A. M.; Solomon, M. T.; Sullivan, S. E.; Singh, M. K.; Sautter, K. E.; Horn, C. P.; Grant, G. D.; Lin, Y.; Wen, J.; Heremans, F. J.; Guha, S.; Awschalom, D. D. Purcell Enhancement of Erbium Ions in TiO<sub>2</sub> on Silicon Nanocavities. *Nano Letters* **2022**, *22*, 6530–6536.
